# Supplementary material for: Knowing About Knowing: An Illusion of Human Competence Can Hinder Appropriate Reliance on AI Systems
Source: arXiv:2301.11333 source file (2023-01-25)
Supplement: Supplementary file 1 [file sec-appendix.tex]

\appendix

\section{Additional Results}
\glcomment{It's also fine that we don't include appendix in revision. In case of word count limit.}
% \glcomment{I also found we have similar results for the second batch of tasks as Table~\ref{tab:hypothesis-res-1-new}. We can add one extra paragraph, table to show it}

\revise{While \textbf{H1} is verified on the first batch of tasks, we are also curious about whether similar conclusion can be drawn from the second batch. In the second batch of tasks, 95 participants showed underestimation of their performance, 59 participants accurately assessed their performance, and 95 participants overestimated themselves. The distribution across each condition is shown in Figure~\ref{fig:participant_distribution_b2}}.

\begin{figure}[htbp]
    \small
    \centering
    \includegraphics[scale=0.37]{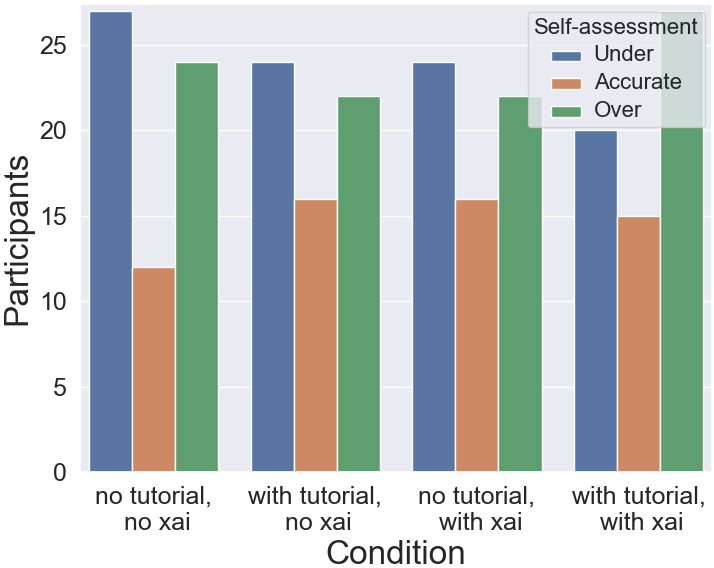}
    \caption{\revise{Distribution of participants with (a) underestimated self-assessment, accurate self-assessment and overestimated self-assessment across all experimental conditions.}}
    \label{fig:participant_distribution_b2}
\end{figure}

\revise{We conducted similar analysis for \textbf{H1} on the second batch of tasks and got consistent results. 
The results are shown in Table~\ref{tab:hypothesis-res-1-b2}. The only exception is that participants with underestimation shows significantly better \textbf{RAIR} when compared to participants with accurate self-assessment.
}

\begin{table}[htbp]
	\centering
	\caption{\revise{Kruskal-Wallis H-test results for inflated self-assessments ( \textbf{H1}) on  reliance-based dependent variables. ``${\dagger\dagger}$'' indicates the effect of variable is significant at the level of 0.0125. ``Under'', ``Accurate'', abd ``Over'' refers to participants who underestimated their performance (miscalibration < 0), accurately estimate their performance (miscalibration = 0), and overestimated their performance (miscalibration > 0) on the second batch of tasks, respectively.}}
	\label{tab:hypothesis-res-1-b2}%
	\begin{small}
	\begin{tabular}{c | c c c c c| c}
	    \hline
	    \textbf{Dependent Variables}& $H$& $p$& $M \pm SD$(Under)& $M \pm SD$(Accurate)& $M \pm SD$(Over)& Post-hoc results\\
	    \hline \hline
	    \textbf{Accuracy}& 108.47& \textbf{<.001}$^{\dagger\dagger}$& $0.72 \pm 0.16$ & $0.55 \pm 0.15$&  $0.41 \pm 0.17$& Under > Accurate > Over\\
	    \rowcolor{gray!15}\textbf{Agreement Fraction}& 22.73& \textbf{<.001}$^{\dagger\dagger}$& $0.74\pm 0.19$& $0.71 \pm 0.21$& $0.59\pm 0.24$& Under, Accurate > Over \\
	\textbf{Switch Fraction}& 16.45& \textbf{<.001}$^{\dagger\dagger}$& $0.55 \pm 0.35$& $0.53 \pm 0.34$& $0.36 \pm 0.31$& Under, Accurate > Over\\
    \rowcolor{gray!15}\textbf{Accuracy-wid}& 72.73& \textbf{<.001}$^{\dagger\dagger}$& $0.65 \pm 0.23$& $0.46 \pm 0.26$& $0.31 \pm 0.22$& Under > Accurate > Over\\
    \textbf{RAIR}& 38.30& \textbf{<.001}$^{\dagger\dagger}$& $0.66 \pm 0.39$& $0.50 \pm 0.37$& $0.31 \pm 0.31$& Under > Accurate > Over\\
	\rowcolor{gray!15}\textbf{RSR}& 17.84& \textbf{<.001}$^{\dagger\dagger}$& $0.55 \pm 0.47$& $0.33 \pm 0.46$& $0.28 \pm 0.45$& Under > Accurate, Over\\
    % \textbf{TiA-Trust}& 3.93& .140& $3.00 \pm 0.81$& $3.22 \pm 0.87$& $3.11 \pm 0.85$& -\\
	    \hline
	\end{tabular}%
	\end{small}
\end{table}

\begin{table}[htbp]
	\centering
	\caption{Correlation with miscalibration with reliance change.\glcomment{we can consider adding this and some extra content to the appendix later.}}
	\label{tab:hypothesis-res-4-zoom}%
	\begin{scriptsize}
	\begin{tabular}{c | c c c c | c c c c}
	    \hline
	     \textbf{Participants}&	\multicolumn{4}{c|}{\textbf{Underestimation}}& \multicolumn{4}{c}{\textbf{Overestimation}}\\
	     \hline
	    \textbf{Dependent Variables}& All& Under $\rightarrow$ Under& Under $\rightarrow$ Accurate& Under $\rightarrow$ Over& All& Over $\rightarrow$ Under& Over $\rightarrow$ Accurate& Over $\rightarrow$ Over\\
	    \hline \hline
	    \textbf{Accuracy}& 25& 7& 10& 8& 25& 12& 5& 8\\
	    \rowcolor{gray!15}\textbf{Accuracy-wid}& 25& 9& 10& 6& 29& 15& 5&9\\
	    \textbf{RAIR}& 19& 4& 7& 8& 21& 10& 5& 6\\
	    \rowcolor{gray!15}\textbf{RSR}& 18& 5& 8& 5& 22& 11& 3& 8\\
	    \hline
	\end{tabular}%
	\end{scriptsize}
\end{table}
